# Supplementary material for: Instanton Theory for Nonadiabatic Tunneling through Near-Barrier Crossings
Source: arXiv:2507.01151 ancillary file (2025-10-20)
Supplement: Supplementary file 1 [file si.pdf]

# Supporting information: Instanton Theory for Nonadiabatic Tunneling through Near-Barrier Crossings

Ziyan Ye,[†] Eric R. Heller,[*,‡] Dong H. Zhang,[¶,§] Jeremy O. Richardson,[*,‖] and Wei Fang[*,†]

†*Department of Chemistry, Shanghai Key Laboratory of Molecular Catalysis and Innovative Materials, State Key Laboratory of Porous Materials for Separation and Conversion, Fudan University, Shanghai 200438, P. R. China*

‡*Department of Chemistry, University of California, Berkeley, 94720 Berkeley, USA*

¶*State Key Laboratory of Molecular Reaction Dynamics, Dalian Institute of Chemical Physics, Chinese Academy of Sciences, Dalian 116023, P. R. China*

§*University of Chinese Academy of Sciences, Beijing 100049, China*

‖*Department of Chemistry and Applied Biosciences, ETH Zürich, Zürich 8093, Switzerland*

E-mail: hellere@berkeley.edu; rjeremy@ethz.ch; wei_fang@fudan.edu.cn

# Contents

**S1 Proof of the necessary condition for the non-convex regime in 1D systems and separable multidimensional systems** **3**

**S2 Singularity cancellation of conjugate points** **5**

**S3 Semiclassical Green's functions in presence of conjugate points** **7**

**S4 Impact of model parameters on rate constant behavior** **9**

S4.1 Double-well plus linear model . . . . . . . . . . . . . . . . . . . . . . . . . . 10

S4.2 Intersecting double-well model . . . . . . . . . . . . . . . . . . . . . . . . . . 11

**References** **14**

# S1 Proof of the necessary condition for the non-convex regime in 1D systems and separable multidimensional systems

We first define the abbreviated action $W_n$ by the line integral

$$W_n \equiv W_n(x_\mathrm{i}, x_\mathrm{f}, E) = \int_{x(q)=x_\mathrm{i}}^{x(q)=x_\mathrm{f}} p_n \, \mathrm{d}q, \tag{S1}$$

where $p_n = \sqrt{2m(V_n - E)}$ is the norm of momentum along the tunneling path. It can be shown to be equivalent to the more commonly used Lagrangian formalism [Eq. (9)] using the Legendre transformation

$$S_n(x_\mathrm{i}, x_\mathrm{f}, \tau_n) = W_n(x_\mathrm{i}, x_\mathrm{f}, E) + E\tau_n. \tag{S2}$$

Differentiating Eq. (S2) gives

$$\frac{\partial^2 S_n}{\partial \boldsymbol{x} \partial \boldsymbol{x}} = \frac{\partial^2 W_n}{\partial \boldsymbol{x} \partial \boldsymbol{x}} - \frac{\partial^2 W_n}{\partial \boldsymbol{x} \partial E} \left( \frac{\partial^2 W_n}{\partial E^2} \right)^{-1} \frac{\partial^2 W_n}{\partial E \partial \boldsymbol{x}}, \tag{S3}$$

where $\boldsymbol{x} \equiv (x', x'')^\mathrm{T}$. Without loss of generality, we assume the trajectory on the reactant surface being on the left-hand side of the hopping point, thus

$$\frac{\partial^2 W}{\partial x' \partial x'} = \frac{\partial^2 W}{\partial x'' \partial x''} = \frac{m \left( g_0^\ddagger - g_1^\ddagger \right)}{p^\ddagger}, \tag{S4}$$

$$\frac{\partial^2 W}{\partial x' \partial x''} = \frac{\partial^2 W}{\partial x'' \partial x'} = 0, \tag{S5}$$

$$\frac{\partial^2 W_0}{\partial x' \partial E} = \frac{\partial^2 W_0}{\partial x'' \partial E} = -\frac{\partial^2 W_1}{\partial x' \partial E} = -\frac{\partial^2 W_1}{\partial x'' \partial E} = -\frac{m}{p^\ddagger}, \tag{S6}$$

where $g_n$ is the gradient on surface $n$, and the superscript $\ddagger$ means that the quantity is evaluated at $x^\ddagger$, the hopping point of instanton.

We first investigate $C_n$ using Eq. (S3) and (S5), given by

$$C_n = \frac{m^2}{p^{\ddagger 2}} \left( \frac{\partial^2 W_n}{\partial E^2} \right)^{-1}, \tag{S7}$$

which can be evaluated explicitly using integration by parts[1]

$$\frac{\partial^2 W_n}{\partial E^2} = \pm \frac{2m}{g_n^\ddagger p^\ddagger} + m \int_{x(q)=x_\mathrm{i}}^{x(q)=x_\mathrm{f}} \frac{H_n}{g_n^2 p_n} \,\mathrm{d}q, \tag{S8}$$

where $H_n$ is the Hessian matrix on surface $n$. N.B. the sign of $\frac{\partial^2 W_n}{\partial E^2}$ is the same as $C_n$, typically positive if $\tau_n > 0$, except that for some strange-shaped PES,[2] the sign is $(-1)^\nu$ with $\nu$ being the number of conjugate points,[3,4] and an extra minus should be counted if $\tau_n < 0$.[5] By Eq. (S8), we find that the sign of it is determined by $\pm g_n^\ddagger$ and $H_n$. In the convex regime, both terms are positive, giving a positive $\frac{\partial^2 W_n}{\partial E^2}$ always. To invert the sign of it, we should either give a negative curvature $H_n$, or even introduce a diabatic barrier to invert the gradient $g_n^\ddagger$. In either case, a negative curvature $H_n$ is necessary.

Then $\boldsymbol{C}$ can be analyzed in a similar manner by combining Eq. (S3)–(S5), with its block entries being

$$\frac{\partial^2 S}{\partial x' \partial x'} = \frac{\partial^2 S}{\partial x'' \partial x''} = \frac{m\left(g_0^\ddagger - g_1^\ddagger\right)}{p^\ddagger} - \frac{m^2}{p^{\ddagger 2}} \left[ \left( \frac{\partial^2 W_0}{\partial E^2} \right)^{-1} + \left( \frac{\partial^2 W_1}{\partial E^2} \right)^{-1} \right], \tag{S9}$$

$$\frac{\partial^2 S}{\partial x' \partial x''} = \frac{\partial^2 S}{\partial x'' \partial x'} = -\frac{m^2}{p^{\ddagger 2}} \left[ \left( \frac{\partial^2 W_0}{\partial E^2} \right)^{-1} + \left( \frac{\partial^2 W_1}{\partial E^2} \right)^{-1} \right], \tag{S10}$$

and since the symmetry in Eq. (S9) and (S10), $\boldsymbol{C}$ can always be block-diagonalized by

transforming coordinates from $x', x''$ to $x_+ = \frac{1}{2}(x' + x''), x_- = x' - x''$ to give

$$\frac{\partial^2 S}{\partial x_+ \partial x_+} = \frac{2m\left(g_0^\ddagger - g_1^\ddagger\right)}{p^\ddagger} - \frac{4m^2}{p^{\ddagger 2}}\left[\left(\frac{\partial^2 W_0}{\partial E^2}\right)^{-1} + \left(\frac{\partial^2 W_1}{\partial E^2}\right)^{-1}\right], \tag{S11}$$

$$\frac{\partial^2 S}{\partial x_- \partial x_-} = \frac{m\left(g_0^\ddagger - g_1^\ddagger\right)}{2p^\ddagger}, \tag{S12}$$

by which we notice that in line with Ref. 5, $\frac{\partial^2 S}{\partial x_- \partial x_-}$ is always positive in the normal regime ($g_0^\ddagger > g_1^\ddagger$), and negative in the inverted regime ($g_0^\ddagger < g_1^\ddagger$), be it the convex regime or non-convex one. Inserting Eq. (S8) into Eq. (S11) gives

$$\frac{\partial^2 S}{\partial x_+ \partial x_+} = \frac{2m^2}{p^\ddagger}\left[\frac{1}{g_0^\ddagger}\left(\frac{\partial^2 W_0}{\partial E^2}\right)^{-1}\int_{x''}^{x'}\frac{H_0}{g_0^2 p_0}\,\mathrm{d}q + \frac{1}{-g_1^\ddagger}\left(\frac{\partial^2 W_1}{\partial E^2}\right)^{-1}\int_{x'}^{x''}\frac{H_1}{g_1^2 p_1}\,\mathrm{d}q\right]. \tag{S13}$$

The sign of $\frac{\partial^2 S}{\partial x_+ \partial x_+}$ is, similar to Eq. (S8), determined by $\pm g_n^\ddagger$, $H_n$, and $\frac{\partial^2 W_n}{\partial E^2}$, which is also determined by the former two terms. The necessary condition for $\frac{\partial^2 S}{\partial x_+ \partial x_+} < 0$ is found to be exactly the same as that for $C_n < 0$.

To briefly summarize, the necessary (but not sufficient) condition for the non-convex regime in 1D systems, defined as the regime where either $C_n$ or $C$ exchanges its minus with $\frac{\mathrm{d}^2 S}{\mathrm{d}\tau^2}$, is a non-convex diabatic PES. In multidimensional systems, we assume that diabatic PESs are non-convex along the instanton path, but that it is convex perpendicular to the path. And this conclusion can be directly applied to separable multidimensional systems, since all dimensions are separated in $C_n$ and $C$.

# S2 Singularity cancellation of conjugate points

According to Eq. (S3), we reformulate $C_n$ as[3,4]

$$C_n = \left(\frac{\partial^2 W_n}{\partial E^2}\right)^{-1}\left|\frac{\partial^2 W_n}{\partial x' \partial E}\frac{\partial^2 W_n}{\partial E \partial x''} - \frac{\partial^2 W_n}{\partial x' \partial x''}\frac{\partial^2 W_n}{\partial E^2}\right|. \tag{S14}$$

If $\Sigma$ also contributes a $\left(\frac{\partial^2 W_n}{\partial E^2}\right)^{-1}$ term, the singularity should cancel out. Taking advantage of the symmetry of $\Sigma$, the symbols in Eq. (13) can be simplified as[4]

$$\Sigma = \begin{vmatrix} \frac{\partial^2 S}{\partial x' \partial x'} & \frac{\partial^2 S}{\partial x' \partial x''} & \frac{\partial^2 S}{\partial x' \partial \tau} \\ \frac{\partial^2 S}{\partial x'' \partial x'} & \frac{\partial^2 S}{\partial x'' \partial x''} & \frac{\partial^2 S}{\partial x'' \partial \tau} \\ \frac{\partial^2 S}{\partial \tau \partial x'} & \frac{\partial^2 S}{\partial \tau \partial x''} & \frac{\partial^2 S}{\partial \tau^2} \end{vmatrix} \equiv \begin{vmatrix} \boldsymbol{A} & \boldsymbol{B} & \boldsymbol{c} \\ \boldsymbol{B} & \boldsymbol{A} & \boldsymbol{c} \\ \boldsymbol{c}^{\mathrm{T}} & \boldsymbol{c}^{\mathrm{T}} & d \end{vmatrix}, \tag{S15}$$

and block-diagonalized as

$$\Sigma = \begin{vmatrix} \boldsymbol{A} - \boldsymbol{B} & \mathbf{O} & \mathbf{0} \\ \mathbf{O} & \boldsymbol{A} + \boldsymbol{B} & \mathbf{0} \\ \mathbf{0}^{\mathrm{T}} & \mathbf{0}^{\mathrm{T}} & d - 2\boldsymbol{c}^{\mathrm{T}} \left(\boldsymbol{A} + \boldsymbol{B}\right)^{-1} \boldsymbol{c} \end{vmatrix}, \tag{S16}$$

where both $\boldsymbol{A}$ and $\boldsymbol{B}$ are symmetric matrices, $\mathbf{O}$ is a square zero matrix, and $\mathbf{0}$ is a zero column vector. First, $\boldsymbol{A} - \boldsymbol{B}$ is irrelevant to $\frac{\partial^2 W_n}{\partial E^2}$, since

$$\boldsymbol{A} - \boldsymbol{B} \equiv \frac{\partial^2 S}{\partial x' \partial x'} - \frac{\partial^2 S}{\partial x' \partial x''} = \frac{\partial^2 W}{\partial x' \partial x'} - \frac{\partial^2 W}{\partial x' \partial x''}. \tag{S17}$$

Then we can write $\boldsymbol{A} + \boldsymbol{B}$ similarly

$$\begin{aligned} \boldsymbol{A} + \boldsymbol{B} &\equiv \frac{\partial^2 S}{\partial x' \partial x'} + \frac{\partial^2 S}{\partial x' \partial x''} \\ &= \frac{\partial^2 W}{\partial x' \partial x'} + \frac{\partial^2 W}{\partial x' \partial x''} - 2\frac{\partial^2 W_0}{\partial x' \partial E}\left(\frac{\partial^2 W_0}{\partial E^2}\right)^{-1}\frac{\partial^2 W_0}{\partial E \partial x'} - 2\frac{\partial^2 W_1}{\partial x' \partial E}\left(\frac{\partial^2 W_1}{\partial E^2}\right)^{-1}\frac{\partial^2 W_1}{\partial E \partial x'}, \end{aligned} \tag{S18}$$

where we use the fact that $\frac{\partial^2 W_n}{\partial x' \partial E} = \frac{\partial^2 W_n}{\partial x'' \partial E}$ to simplify the equation. Apparently, $|\boldsymbol{A} + \boldsymbol{B}|$ is asymptotic to $\left(\frac{\partial^2 W_n}{\partial E^2}\right)^{-1}$. $d$ and $\boldsymbol{c}$ are given by[4]

$$d \equiv \frac{\partial^2 S}{\partial \tau^2} = -\left(\frac{\partial^2 W_0}{\partial E^2}\right)^{-1} - \left(\frac{\partial^2 W_1}{\partial E^2}\right)^{-1}, \tag{S19}$$

$$\boldsymbol{c} \equiv \frac{\partial^2 S}{\partial x' \partial \tau} = \frac{\partial^2 W_0}{\partial x' \partial E} \left( \frac{\partial^2 W_0}{\partial E^2} \right)^{-1} - \frac{\partial^2 W_1}{\partial x' \partial E} \left( \frac{\partial^2 W_1}{\partial E^2} \right)^{-1}. \tag{S20}$$

Without loss of generality, we assume that the conjugate point is found on $V_0$, so in the following, we only focus on the leading terms with the factor $\left(\frac{\partial^2 W_0}{\partial E^2}\right)^{-1}$. The second term of the last diagonal entry in Eq. (S16) is then obtained as

$$\begin{aligned} \boldsymbol{c}^{\mathrm{T}} \left( \boldsymbol{A} + \boldsymbol{B} \right)^{-1} \boldsymbol{c} &\sim \frac{\partial^2 W_0}{\partial x' \partial E} \left( \frac{\partial^2 W_0}{\partial E^2} \right)^{-1} \left[ -2 \frac{\partial^2 W_0}{\partial x' \partial E} \left( \frac{\partial^2 W_0}{\partial E^2} \right)^{-1} \frac{\partial^2 W_0}{\partial E \partial x'} \right]^{-1} \left( \frac{\partial^2 W_0}{\partial E^2} \right)^{-1} \frac{\partial^2 W_0}{\partial E \partial x'} \\ &= -\frac{1}{2} \left( \frac{\partial^2 W_0}{\partial E^2} \right)^{-1}, \end{aligned} \tag{S21}$$

which happens to cancel with the first term in Eq. (S19), leaving the entry being

$$d - 2\boldsymbol{c}^{\mathrm{T}} \left( \boldsymbol{A} + \boldsymbol{B} \right)^{-1} \boldsymbol{c} = -\left( \frac{\partial^2 W_1}{\partial E^2} \right)^{-1}, \tag{S22}$$

which is not singular.

In summary, although singularity encountered in $C_n$ when a trajectory ends up at its conjugate point, it cancels exactly with that from $\boldsymbol{A} + \boldsymbol{B}$, i.e. $\frac{\partial^2 S}{\partial x_+ \partial x_+}$, giving an analytic prefactor $\frac{C_0 C_1}{\Sigma}$.

# S3 Semiclassical Green's functions in presence of conjugate points

Similar to the propagators, the Green's function can be approximated semiclassically by

$$\mathrm{Im} G_n(x_{\mathrm{i}}, x_{\mathrm{f}}, E) \sim -\frac{\pi}{(2\pi\hbar)^{(f+1)/2}} \sqrt{D_n}\, \mathrm{e}^{-W_n/\hbar}, \tag{S23}$$

where the prefactor $D_n$ is defined by an $(f+1)$-dimensional determinant

$$D_n = (-1)^{f+1} \begin{vmatrix} \frac{\partial^2 W_n}{\partial x_{\rm i} \partial x_{\rm f}} & \frac{\partial^2 W_n}{\partial x_{\rm i} \partial E} \\ \frac{\partial^2 W_n}{\partial E \partial x_{\rm f}} & \frac{\partial^2 W_n}{\partial E^2} \end{vmatrix} . \tag{S24}$$

Given a trajectory with a conjugate point, we may use the composition property of the propagator to break up the path into two segments, neither of which has a conjugate point. Define an intermediate point $x$ somewhere along the trajectory (avoid turning points and make sure it's far enough away from $x_{\rm i}$ and $x_{\rm f}$ such that it will fix the sign problem). The complex time of two segments $a$ and $b$ is denoted by $\tau_a + {\rm i}t_a$ and $\tau_b + {\rm i}t_b$ such that $\tau_a + \tau_b = \tau$ and $t_a + t_b = t$. If we approximate the propagators by van-Vleck semiclassical propagators,[1,3] the composition property gives[6]

$$K_n(x_{\rm i}, x_{\rm f}, \tau + {\rm i}t) = \int K_n(x_{\rm i}, x, \tau_a + {\rm i}t_a) K_n(x, x_{\rm f}, \tau_b + {\rm i}t_b)\, {\rm d}x \tag{S25}$$

$$\sim \int \sqrt{\frac{C_a}{(2\pi\hbar)^f}} \sqrt{\frac{C_b}{(2\pi\hbar)^f}}\, {\rm e}^{-(S_a+S_b)/\hbar}\, {\rm d}x, \tag{S26}$$

and the prefactors are related by[3,7]

$$C_n = C_a C_b \left| \frac{\partial^2 (S_a + S_b)}{\partial x \partial x} \right|^{-1}, \tag{S27}$$

where the derivative is evaluated at the stationary points of $S_a$ and $S_b$ w.r.t $x$. We cannot apply steepest-descent approximation to Eq. (S26) since $\frac{\partial^2 (S_a+S_b)}{\partial x \partial x} < 0$. Nonetheless, as we will show, these saddle-point paths can be important for the Green's functions.

The Green's function is defined by the transformation[3]

$$G(x_{\rm i}, x_{\rm f}, E) = \frac{1}{2{\rm i}\hbar} \int_{-\infty}^{+\infty} K_n(x_{\rm i}, x_{\rm f}, \tau + {\rm i}t)\, {\rm e}^{E(\tau+{\rm i}t)/\hbar}\, {\rm d}t. \tag{S28}$$

To obtain the semiclassical Green's functions in presence of conjugate points, we first break

the propagator into two parts

$$G\left(x_{\mathrm{i}}, x_{\mathrm{f}}, E\right) \sim \frac{1}{2\mathrm{i}\hbar} \iint_{-\infty}^{+\infty} \sqrt{\frac{C_a}{(2\pi\hbar)^f}} \sqrt{\frac{C_b}{(2\pi\hbar)^f}}\, \mathrm{e}^{-(S_a+S_b)/\hbar + E(\tau+\mathrm{i}t)/\hbar}\, \mathrm{d}x\, \mathrm{d}t, \tag{S29}$$

and do the steepest-descent integration over $x$ and $t$ together

$$\mathrm{Im}G\left(x_{\mathrm{i}}, x_{\mathrm{f}}, E\right) \sim -\frac{\pi}{(2\pi\hbar)^{(f+1)/2}} \frac{\sqrt{C_a}\sqrt{C_b}}{\sqrt{-\left|\nabla^2_{x,\tau}(S_a+S_b)\right|}}\, \mathrm{e}^{-(S_a+S_b)/\hbar + E\tau/\hbar} \tag{S30}$$

$$= -\frac{\pi}{(2\pi\hbar)^{(f+1)/2}} \sqrt{\frac{C_a C_b}{-\frac{\mathrm{d}^2(S_a+S_b)}{\mathrm{d}\tau^2}\left|\frac{\partial^2(S_a+S_b)}{\partial x \partial x}\right|}}\, \mathrm{e}^{-(S_a+S_b)/\hbar + E\tau/\hbar} \tag{S31}$$

$$= -\frac{\pi}{(2\pi\hbar)^{(f+1)/2}} \sqrt{\frac{C_n}{-\frac{\partial^2 S_n}{\partial \tau^2}}}\, \mathrm{e}^{-S_n/\hbar + E\tau/\hbar} \tag{S32}$$

$$= -\frac{\pi}{(2\pi\hbar)^{(f+1)/2}} \sqrt{D_n}\, \mathrm{e}^{-W_n/\hbar}, \tag{S33}$$

where every term inside the square roots in Eq. (S30) is positive since we break the original trajectory into two stable ones. Note the differences between full and partial derivatives. Equation (S33) has exactly the same form as Eq. (S23), so Green's functions still behave well in the non-convex regime. Combined with the derivation of instanton theory via Green's functions,[4] this justifies the use of instanton theory for paths with conjugate points.

# S4 Impact of model parameters on rate constant behavior

In this section, we will demonstrate how $k(\beta)$ depends on the coupling $\Delta$ and the position of the crossing point $x^{\ddagger}$. $x^{\ddagger}$ is controlled by $\varepsilon_1$, the bias of $V_1$. A direct scaling of the space coordinates or the potential energy of the system affects the scanning results by simply scaling the curves correspondingly.

## S4.1 Double-well plus linear model

A stronger coupling moves the curve of the concerted mechanism upwards, making this mechanism more favorable. And if $x^‡$ is closer to TS, the concerted mechanism is also more favorable, while it has little effect on the sequential mechanism.

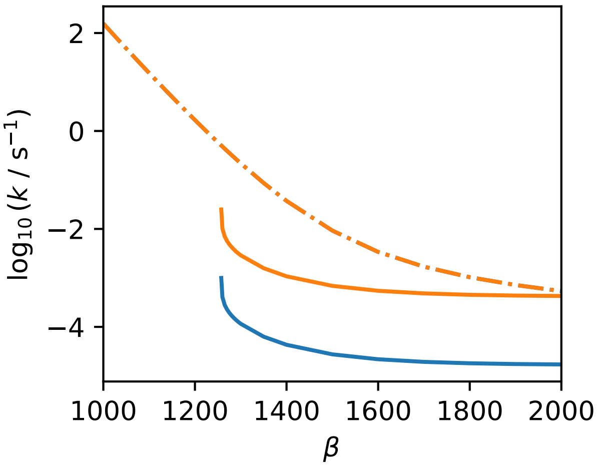


(a)

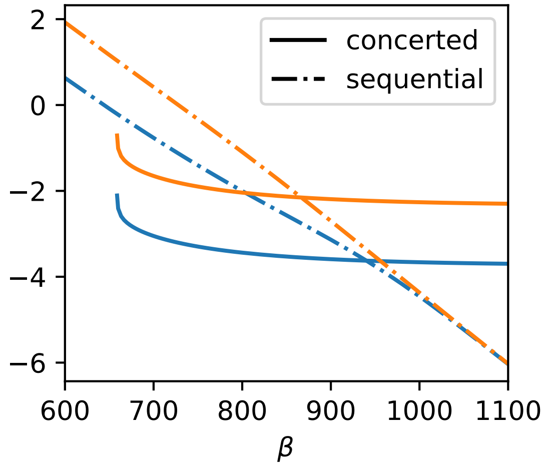


(b)

Figure S1: Overall rate constants $k$ of two mechanisms for model A (a) and model B (b) as a function of inverse temperature $\beta$. The concerted mechanism, shown as solid lines, is compared with the sequential mechanism shown as dash-dot lines. The blue set is for $\Delta = 0.0001$, and the orange set is for $\Delta = 0.0005$. In panel a, the blue dash-dot line overlaps with the orange one.

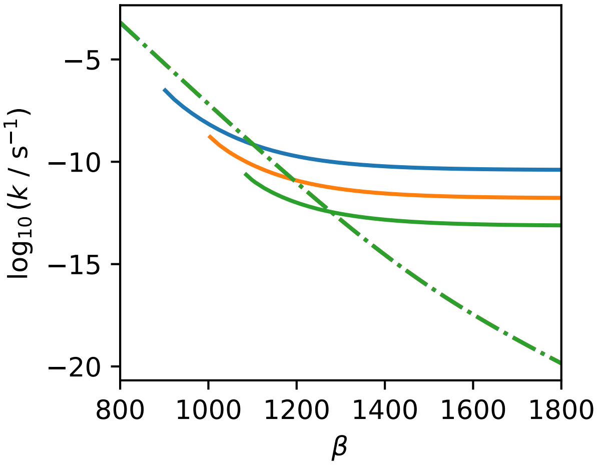


(a)

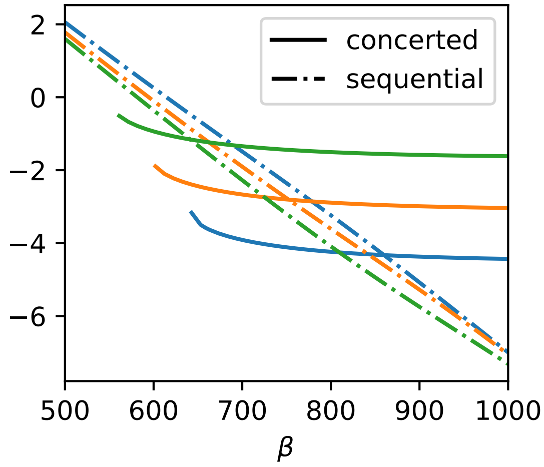


(b)

Figure S2: Overall rate constants $k$ of two mechanisms for model A (a) and model B (b) as a function of inverse temperature $\beta$. The concerted mechanism, shown as solid lines, is compared with the sequential mechanism shown as dash-dot lines. The position of the crossing point $x^\ddagger$ is controlled by setting different $\varepsilon_1$. $\varepsilon_1$ in blue, orange and green sets are (a) 0.07, 0.08, 0.09, and (b) 0.01, 0.02, 0.03 respectively. In panel a, the orange dash-dot line overlaps with the green one.

## S4.2 Intersecting double-well model

Another model we choose here is two quartic double-well potentials intersecting each other, given by

$$V_0 = \lambda \left(\frac{x}{\xi} + 1\right)^2 \left(\frac{x}{\xi} - 1\right)^2 + \kappa_0 x + \varepsilon_0, \tag{S34}$$

$$V_1 = \lambda \left(\frac{x}{\xi} + 1\right)^2 \left(\frac{x}{\xi} - 1\right)^2 + \kappa_1 x + \varepsilon_1, \tag{S35}$$

with $m = 1$ amu, $\lambda = 0.06$, $\xi = 2$, $\kappa_0 = 0.005$, $\varepsilon_0 = 0.01$, $\kappa_1 = -0.015$, $\varepsilon_1 = 0.02$, and $\Delta = 0.0004$ in atomic units. The parameter dependence is qualitatively the same as that in model A, i.e., a stronger coupling and a smaller distance between the TS and the MECP favor the concerted mechanism.

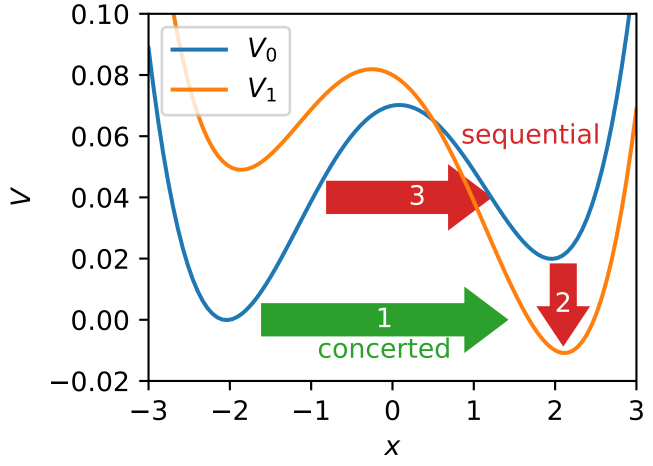


Figure S3: Diabatic potential-energy curves of a system with two quartic double-well potentials crossing each other. The arrows annotate two possible reaction mechanisms from the reactant side to the product side.

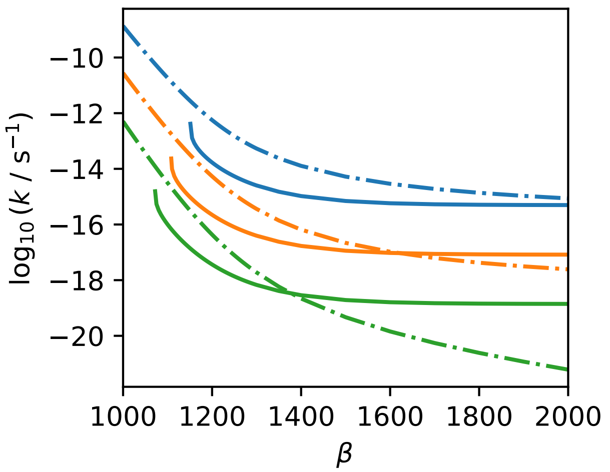


Figure S4: Overall rate constants $k$ of two mechanisms for intersecting double-well as a function of inverse temperature $\beta$. The concerted mechanism, shown as solid lines, is compared with the sequential mechanism shown as dash-dot lines. The blue set is for $\kappa_0 = -0.002$, the orange set is for $\kappa_0 = 0$, and the green set is for $\kappa_0 = 0.002$.

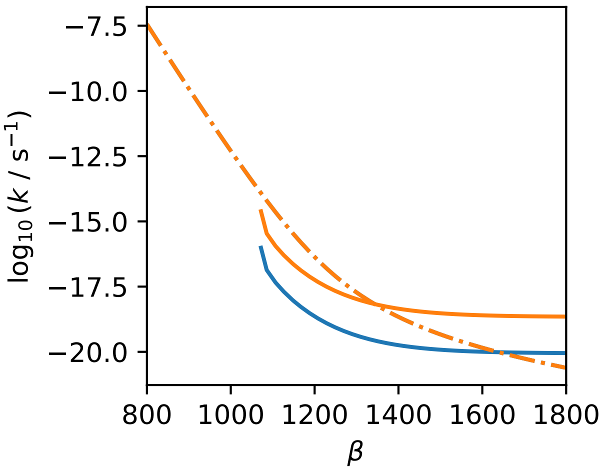


Figure S5: Overall rate constants $k$ of two mechanisms for intersecting double-well as a function of inverse temperature $\beta$. The concerted mechanism, shown as solid lines, is compared with the sequential mechanism shown as dash-dot lines. The blue set is for $\Delta = 0.0001$, and the orange set is for $\Delta = 0.0005$. The blue dash-dot line overlaps with the orange one.

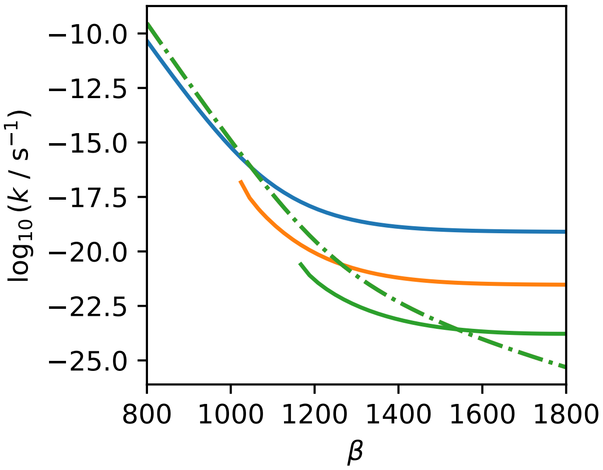


Figure S6: Overall rate constants $k$ of two mechanisms for intersecting double-well as a function of inverse temperature $\beta$. The concerted mechanism, shown as solid lines, is compared with the sequential mechanism shown as dash-dot lines. The position of the crossing point $x^\ddagger$ is controlled by setting different $\varepsilon_1$. $\varepsilon_1$ in blue, orange and green sets are 0.01, 0.02, 0.03 respectively. The blue and orange dash-dot lines overlap with the green one.

# References


(1) Miller, W. H. Classical path approximation for the Boltzmann density matrix. *J. Chem. Phys.* **1971**, *55*, 3146–3149.

(2) Fang, W.; Richardson, J. O.; Chen, J.; Li, X.-Z.; Michaelides, A. Simultaneous deep tunneling and classical hopping for hydrogen diffusion on metals. *Phys. Rev. Lett.* **2017**, *119*, 126001.

(3) Gutzwiller, M. C. In *Chaos in Classical and Quantum Mechanics*; John, F., Kadanoff, L., Marsden, J. E., Sirovich, L., Wiggins, S., Eds.; Interdisciplinary Applied Mathematics; Springer New York: New York, NY, 1990; Vol. 1.

(4) Richardson, J. O.; Bauer, R.; Thoss, M. Semiclassical Green's functions and an instanton formulation of electron-transfer rates in the nonadiabatic limit. *J. Chem. Phys.* **2015**, *143*, 134115.

(5) Heller, E. R.; Richardson, J. O. Instanton formulation of Fermi's golden rule in the Marcus inverted regime. *J. Chem. Phys.* **2020**, *152*, 034106.

(6) Feynman, R. P.; Hibbs, A. R. *Quantum Mechanics and Path Integrals*, 20th ed.; International Series in Pure and Applied Physics; McGraw-Hill: New York, NY, 1995.

(7) Richardson, J. O. Ring-polymer instanton theory. *Int. Rev. Phys. Chem.* **2018**, *37*, 171–216.
